# Supplementary material for: CoBe -- Coded Beacons for Localization, Object Tracking, and SLAM Augmentation
Source: arXiv:1708.05625 ancillary file (2020-04-21)
Supplement: Supplementary file 1 [file winqi-anc.pdf]

# Winqi: A System for 6D Localization and SLAM Augmentation Using Wideangle Optics and Coded Light Beacons,

## Code tables

Aaron Wetzler    Ron Kimmel

twerd@cs.technion.ac.il    ron@cs.technion.ac.il

Technion, Israel Institute of Technology

### 1. Winqi videos

The following videos shows a video of red/green visible light codes:

[www.youtube.com/watch?v=3rT0Gz-WH8w](http://www.youtube.com/watch?v=3rT0Gz-WH8w)

The following video illustrates a use case with a wideangle camera or light blob sensor on both a VR mask and VR controller.

[www.youtube.com/watch?v=B0v4j49PV7A](http://www.youtube.com/watch?v=B0v4j49PV7A)

### 2. Code tables

Table 1. 7-bit codes. Total : 2

|    |         |
|----|---------|
| 7  | 0000111 |
| 63 | 0111111 |

Table 2. 8-bit codes. Total : 4

|     |          |
|-----|----------|
| 7   | 00000111 |
| 51  | 00110011 |
| 85  | 01010101 |
| 127 | 01111111 |

Table 3. 9-bit codes. Total : 3

|     |           |
|-----|-----------|
| 7   | 000000111 |
| 51  | 000110011 |
| 127 | 001111111 |

Table 4. 10-bit codes. Total : 5

|     |            |
|-----|------------|
| 7   | 0000000111 |
| 51  | 0000110011 |
| 85  | 0001010101 |
| 127 | 0001111111 |
| 439 | 0110110111 |

Table 5. 11-bit codes. Total : 6

|     |             |
|-----|-------------|
| 7   | 00000000111 |
| 51  | 00000110011 |
| 85  | 00001010101 |
| 127 | 00001111111 |
| 335 | 00101001111 |
| 887 | 01101110111 |

Table 6. 12-bit codes. Total : 8

|      |              |
|------|--------------|
| 7    | 000000000111 |
| 51   | 000000110011 |
| 85   | 000001010101 |
| 127  | 000001111111 |
| 273  | 000100010001 |
| 335  | 000101001111 |
| 887  | 001101110111 |
| 2047 | 011111111111 |

Table 7. 13-bit codes. Total : 12

|      |               |
|------|---------------|
| 7    | 000000000111  |
| 51   | 0000000110011 |
| 85   | 0000001010101 |
| 127  | 0000001111111 |
| 265  | 0000100001001 |
| 335  | 0000101001111 |
| 467  | 0000111010011 |
| 749  | 0001011101101 |
| 891  | 0001101111011 |
| 1207 | 0010010110111 |
| 1951 | 0011110011111 |
| 2815 | 0101011111111 |

Table 8. 14-bit codes. Total : 15

|      |                |
|------|----------------|
| 7    | 000000000111   |
| 51   | 00000000110011 |
| 85   | 00000001010101 |
| 127  | 00000001111111 |
| 265  | 0000100001001  |
| 335  | 0000101001111  |
| 467  | 00000111010011 |
| 741  | 00001011100101 |
| 959  | 0000111011111  |
| 1207 | 00010010110111 |
| 1845 | 00011100110101 |
| 1935 | 00011110001111 |
| 2811 | 00101011111011 |
| 4063 | 00111111011111 |
| 5461 | 01010101010101 |

Table 9. 15-bit codes. Total : 25

|       |                 |
|-------|-----------------|
| 7     | 00000000000111  |
| 51    | 000000000110011 |
| 85    | 000000001010101 |
| 127   | 000000001111111 |
| 265   | 000000100001001 |
| 335   | 000000101001111 |
| 467   | 000000111010011 |
| 741   | 000001011100101 |
| 959   | 00000110111111  |
| 1207  | 000010010110111 |
| 1415  | 000010110000111 |
| 1583  | 000011000101111 |
| 1753  | 000011011011001 |
| 2007  | 000011111010111 |
| 2211  | 000100010100011 |
| 2293  | 000100011110101 |
| 2733  | 000101010101101 |
| 2875  | 000101100111011 |
| 3327  | 000110011111111 |
| 4685  | 001001001001101 |
| 5503  | 001010101111111 |
| 6991  | 001101101001111 |
| 8127  | 001111110111111 |
| 11191 | 010101110110111 |
| 15855 | 011110111101111 |

Table 10. 16-bit codes. Total : 35

|       |                  |
|-------|------------------|
| 7     | 000000000000111  |
| 51    | 0000000000110011 |
| 85    | 0000000001010101 |
| 127   | 0000000001111111 |
| 265   | 0000000100001001 |
| 335   | 0000000101001111 |
| 467   | 0000000111010011 |
| 741   | 0000001011100101 |
| 771   | 0000001100000011 |
| 959   | 0000001110111111 |
| 1187  | 0000010010100011 |
| 1245  | 0000010011011101 |
| 1567  | 0000011000011111 |
| 1935  | 0000011110001111 |
| 1961  | 0000011110101001 |
| 2263  | 0000100011010111 |
| 2367  | 0000100100111111 |
| 2599  | 0000101000100111 |
| 2867  | 0000101100110011 |
| 3177  | 0000110001101001 |
| 3373  | 0000110100101101 |
| 3551  | 0000110111011111 |
| 4045  | 0000111111001101 |
| 4827  | 0001001011011011 |
| 5289  | 0001010010101001 |
| 5975  | 0001011101010111 |
| 6131  | 0001011111110011 |
| 6635  | 0001100111101011 |
| 7807  | 0001111001111111 |
| 9807  | 0010011001001111 |
| 10939 | 0010101010111011 |
| 14335 | 0011011111111111 |
| 14813 | 0011100111011101 |
| 16341 | 0011111111010101 |
| 23419 | 0101101101111011 |

Table 11. 17-bit codes. Total : 52

|       |                    |
|-------|--------------------|
| 7     | 0000000000000111   |
| 51    | 0000000000110011   |
| 85    | 0000000001010101   |
| 127   | 0000000001111111   |
| 265   | 0000000100001001   |
| 335   | 0000000101001111   |
| 467   | 0000000111010011   |
| 741   | 00000001011100101  |
| 771   | 00000001100000011  |
| 959   | 00000001110111111  |
| 1187  | 00000010010100011  |
| 1245  | 00000010011011101  |
| 1567  | 00000011000011111  |
| 1927  | 00000011110000111  |
| 1961  | 00000011110101001  |
| 2019  | 00000011111100011  |
| 2263  | 00000100011010111  |
| 2367  | 00000100100111111  |
| 2599  | 00000101000100111  |
| 2833  | 00000101100010001  |
| 3177  | 00000110001101001  |
| 3371  | 00000110100101011  |
| 3535  | 00000110111001111  |
| 4087  | 00000111111110111  |
| 4283  | 00001000010111011  |
| 4461  | 00001000101101101  |
| 4637  | 00001001000011101  |
| 4915  | 00001001100110011  |
| 5611  | 00001010111101011  |
| 5855  | 00001011011011111  |
| 6399  | 00001100011111111  |
| 6481  | 00001100101010001  |
| 7743  | 00001111000111111  |
| 8027  | 00001111101011011  |
| 9103  | 00010001110001111  |
| 9975  | 000100011011110111 |
| 10173 | 000100011110111101 |
| 10853 | 00010101001100101  |
| 10927 | 00010101010101111  |
| 12025 | 00010111101111001  |
| 12959 | 00011001010011111  |
| 13031 | 00011001011100111  |
| 14157 | 00011011101001101  |
| 14781 | 00011100110111101  |
| 15359 | 00011101111111111  |
| 18795 | 00100100101101011  |
| 20205 | 00100111011101101  |
| 23167 | 00101101001111111  |
| 24271 | 00101111011001111  |
| 44895 | 01010111101011111  |
| 56247 | 01101101110110111  |
| 65023 | 01111110111111111  |

Table 12. 18-bit codes. Total : 83

|        |                     |
|--------|---------------------|
| 7      | 00000000000000111   |
| 51     | 00000000000110011   |
| 85     | 00000000001010101   |
| 127    | 00000000001111111   |
| 265    | 00000000100001001   |
| 335    | 00000000101001111   |
| 467    | 0000000011010011    |
| 741    | 000000001011100101  |
| 771    | 00000001100000011   |
| 959    | 00000001110111111   |
| 1187   | 00000010010100011   |
| 1245   | 00000010011011101   |
| 1567   | 00000011000011111   |
| 1927   | 00000011110000111   |
| 1961   | 00000011110101001   |
| 2019   | 0000001111100011    |
| 2263   | 00000100011010111   |
| 2367   | 00000100100111111   |
| 2599   | 00000101000100111   |
| 2833   | 00000101100010001   |
| 3177   | 00000110001101001   |
| 3371   | 00000110100101011   |
| 3535   | 00000110110011111   |
| 4087   | 00000111111101111   |
| 4283   | 00001000010111011   |
| 4461   | 00001000101101101   |
| 4631   | 00001001000010111   |
| 4901   | 00001001100100101   |
| 5427   | 0000101001100110011 |
| 5627   | 00001010111111011   |
| 5975   | 00001011101010111   |
| 6427   | 00001100100011011   |
| 6631   | 00001100111100111   |
| 6841   | 00001101010111001   |
| 7367   | 00001110011000111   |
| 7605   | 00001110110110101   |
| 7743   | 00001111000111111   |
| 8733   | 000010001000011101  |
| 9001   | 000010001100101001  |
| 9557   | 000010010101010101  |
| 9631   | 00001001011001111   |
| 9907   | 000010011010110011  |
| 10205  | 000010011111011101  |
| 10467  | 000010100011100011  |
| 10887  | 000010101010000111  |
| 11647  | 000010110101111111  |
| 12107  | 000010111101001011  |
| 12527  | 000011000011101111  |
| 12913  | 000011001001110001  |
| 14271  | 000011011110111111  |
| 15277  | 000011101110101101  |
| 15571  | 000011110011010011  |
| 15973  | 000011111001100101  |
| 16371  | 00001111111110011   |
| 17759  | 00010001010101111   |
| 18391  | 000100011111010111  |
| 18857  | 000100100110101001  |
| 19339  | 000100101110001011  |
| 20457  | 00010011111101001   |
| 20927  | 000101000110111111  |
| 21195  | 000101001011001011  |
| 22107  | 000101011001011011  |
| 22773  | 000101100011110101  |
| 24419  | 000101111101100011  |
| 24543  | 00010111111011111   |
| 26205  | 000110011001011101  |
| 27189  | 000110101000110101  |
| 29359  | 000111001010101111  |
| 29641  | 000111001111001001  |
| 29919  | 000111010011011111  |
| 30439  | 000111011011100111  |
| 39355  | 001001100110111011  |
| 39503  | 001001101001001111  |
| 43741  | 001010101011011101  |
| 46835  | 001011011011110011  |
| 48107  | 001011101111101011  |
| 48759  | 001011110001110111  |
| 52567  | 001100110101010111  |
| 55807  | 001101100111111111  |
| 61429  | 001110111111110101  |
| 62957  | 001111010111101101  |
| 65279  | 001111110111111111  |
| 128991 | 011111011111011111  |

Table 13. 19-bit codes. Total : 138

|       |                      |        |                      |
|-------|----------------------|--------|----------------------|
| 7     | 00000000000000000111 | 39637  | 0001001101011010101  |
| 51    | 0000000000000110011  | 40047  | 0001001110001101111  |
| 85    | 0000000000001010101  | 40823  | 0001001111011101111  |
| 127   | 0000000000011111111  | 40953  | 0001001111111111001  |
| 265   | 000000000100001001   | 41725  | 0001010001011111101  |
| 335   | 000000000101001111   | 42707  | 0001010011011010011  |
| 467   | 000000000111010011   | 42837  | 0001010011101010101  |
| 741   | 000000001011100101   | 43699  | 0001010101010110011  |
| 771   | 00000000110000011    | 44269  | 0001010110011101101  |
| 959   | 000000001110111111   | 45039  | 0001010111111101111  |
| 1187  | 000000010010100011   | 45991  | 0001011001110100111  |
| 1245  | 000000010011011101   | 46269  | 0001011010010111101  |
| 1567  | 000000011000011111   | 48383  | 0001011110011111111  |
| 1927  | 000000011110000111   | 48539  | 0001011111011001101  |
| 1961  | 000000011110101001   | 51709  | 0001100100111111101  |
| 2019  | 00000001111100011    | 51917  | 0001100101011001101  |
| 2263  | 000000010001101011   | 53999  | 0001101001011101111  |
| 2367  | 000000010010011111   | 54093  | 0001101001101001101  |
| 2571  | 0000000101000001011  | 55543  | 0001101100011110111  |
| 2867  | 0000000101100110011  | 56821  | 0001101110111110101  |
| 3177  | 0000000110001101001  | 58303  | 0001110001110111111  |
| 3345  | 0000000110100010001  | 59113  | 0001110011011101001  |
| 3419  | 0000000110101011011  | 61371  | 0001110111110111011  |
| 3663  | 0000000111001001111  | 62031  | 0001111001001001111  |
| 4063  | 000000011111011111   | 63039  | 0001111011000111111  |
| 4283  | 0000001000010111011  | 63197  | 0001111011011011101  |
| 4461  | 0000001000101101101  | 63801  | 0001111100100111001  |
| 4637  | 0000001001000011101  | 63847  | 0001111100101100111  |
| 4901  | 0000001001100100101  | 64841  | 00011111110101001001 |
| 5191  | 0000001010001000111  | 65389  | 00011111111101101101 |
| 5289  | 0000001010010101001  | 77229  | 0010010110110101101  |
| 5611  | 0000001010111101011  | 81231  | 0010011110101001111  |
| 6399  | 0000001100011111111  | 84851  | 0010100101101110011  |
| 6595  | 0000001100111000011  | 89079  | 0010101101111110111  |
| 6969  | 0000001101100111001  | 94079  | 0010110111101111111  |
| 7563  | 0000001110110001011  | 106165 | 0011001111010110101  |
| 7735  | 0000001111000110111  | 106495 | 0011001111111111111  |
| 7747  | 0000001111001000011  | 109533 | 0011010101111011101  |
| 8165  | 0000001111111100101  | 110271 | 0011010111010111111  |
| 8719  | 0000010001000001111  | 113375 | 0011011101011011111  |
| 9001  | 0000010001100101001  | 113899 | 0011011110011101011  |
| 9425  | 0000010010011010001  | 118751 | 0011100111111011111  |
| 9559  | 0000010010101010111  | 177583 | 0101011010110101111  |
| 10045 | 0000010011100111101  | 195583 | 0101111101111111111  |
| 10187 | 0000010011111001011  |        |                      |
| 10339 | 0000010100001100011  |        |                      |
| 10535 | 0000010100100100111  |        |                      |
| 10719 | 0000010100111011111  |        |                      |
| 10953 | 00000101010111001001 |        |                      |
| 11717 | 0000010110111000101  |        |                      |
| 11819 | 0000010111000101011  |        |                      |
| 12587 | 0000011000100101011  |        |                      |
| 13167 | 0000011001101101111  |        |                      |
| 13375 | 0000011010000111111  |        |                      |
| 13965 | 0000011011010001101  |        |                      |
| 14261 | 0000011011110110101  |        |                      |
| 14513 | 0000011100010110001  |        |                      |
| 14995 | 0000011101010010011  |        |                      |
| 15101 | 0000011101011111101  |        |                      |
| 16059 | 0000011111010111011  |        |                      |
| 16271 | 0000011111110001111  |        |                      |
| 16383 | 0000011111111111111  |        |                      |
| 17531 | 0000100010001111011  |        |                      |
| 17585 | 0000100010010110001  |        |                      |
| 17991 | 0000100011001000111  |        |                      |
| 18381 | 0000100011111001101  |        |                      |
| 19327 | 0000100101101111111  |        |                      |
| 19507 | 0000100110000110011  |        |                      |
| 20131 | 0000100111010100011  |        |                      |
| 20185 | 0000100111011011001  |        |                      |
| 21131 | 0000101001010001011  |        |                      |
| 21753 | 00001010100111111001 |        |                      |
| 21773 | 0000101010100001101  |        |                      |
| 22735 | 0000101100011001111  |        |                      |
| 22877 | 0000101100101011101  |        |                      |
| 23271 | 0000101101011100111  |        |                      |
| 23845 | 00001011110100100101 |        |                      |
| 24383 | 0000101111100111111  |        |                      |
| 24425 | 00001011111101101001 |        |                      |
| 25051 | 0000110000111011011  |        |                      |
| 25315 | 00001100010111100011 |        |                      |
| 26231 | 0000110011001111011  |        |                      |
| 26611 | 0000110011111110011  |        |                      |
| 27295 | 0000110101010011111  |        |                      |
| 27599 | 0000110101111001111  |        |                      |
| 27601 | 0000110101111010001  |        |                      |
| 29577 | 0000111001110001001  |        |                      |
| 29787 | 0000111010001011011  |        |                      |
| 30551 | 0000111011101010111  |        |                      |
| 31125 | 0000111100110010101  |        |                      |
| 31475 | 00001111010111110011 |        |                      |
| 35231 | 0001000100110011111  |        |                      |
| 35799 | 0001000101111010111  |        |                      |
| 38491 | 0001001011001011011  |        |                      |

Table 14. 20-bit codes. Total : 231

|       |                       |        |                       |        |                      |
|-------|-----------------------|--------|-----------------------|--------|----------------------|
| 7     | 000000000000000111    | 28571  | 000001011110011011    | 104859 | 00011001100110011011 |
| 51    | 0000000000000110011   | 29007  | 0000011000101001111   | 109359 | 00011010101100101111 |
| 85    | 0000000000001010101   | 29301  | 0000011001001110101   | 110261 | 00011010111010110101 |
| 127   | 0000000000001111111   | 29689  | 00000110011111111001  | 111999 | 00011011010101111111 |
| 265   | 0000000000100001001   | 29725  | 0000011010000011101   | 113977 | 00011011110100111001 |
| 335   | 0000000000101001111   | 29993  | 0000011010100101001   | 118415 | 0001100111010001111  |
| 467   | 0000000000111010011   | 30439  | 0000011011011100111   | 118717 | 0001100111110111101  |
| 741   | 00000000001011100101  | 31343  | 0000011101001101111   | 119463 | 0001101001010100111  |
| 771   | 00000000001100000011  | 31723  | 00000111101111101011  | 120063 | 0001101010111111111  |
| 959   | 0000000000111011111   | 31833  | 00000111110001011001  | 121701 | 0001101101101100101  |
| 1187  | 00000000010010100011  | 33825  | 00001000010000100001  | 122043 | 0001101110010111011  |
| 1245  | 0000000001001101101   | 34283  | 00001000010111101011  | 122839 | 0001101111111010111  |
| 1567  | 00000000011000011111  | 34447  | 00001000011010001111  | 125875 | 00011110101110110011 |
| 1927  | 00000000011110000111  | 34595  | 00001000011100100011  | 126359 | 00011110110110010111 |
| 1961  | 00000000011110101001  | 35125  | 00001000100100110101  | 128831 | 00011111011100111111 |
| 2019  | 00000000011111100011  | 36165  | 00001000110101000101  | 129013 | 0001111101111110101  |
| 2263  | 00000000100011010111  | 36407  | 00001000111000110111  | 130287 | 0001111111001101111  |
| 2367  | 00000000100100111111  | 36837  | 000010001111111100101 | 150461 | 00100100101110111101 |
| 2571  | 00000000101000001011  | 37143  | 00001001000100010111  | 155339 | 0010010111101001011  |
| 2833  | 00000000101100010001  | 37365  | 00001001000111110101  | 157503 | 00100110011100111111 |
| 3173  | 00000000110001100101  | 37723  | 00001001001101011011  | 158893 | 00100110110010101101 |
| 3373  | 00000000110100101101  | 39287  | 00001001100101110111  | 161115 | 00100111010101011011 |
| 3535  | 00000000110111001111  | 39545  | 00001001101001111001  | 169429 | 00101001010111010101 |
| 3771  | 00000000111010111011  | 40029  | 00001001110001011101  | 171855 | 00101001111101001111 |
| 4095  | 00000000111111111111  | 41831  | 00001010001101100111  | 175611 | 00101010101111111011 |
| 4283  | 00000001000010111011  | 42039  | 00001010010000110111  | 179445 | 00101011110011110101 |
| 4461  | 00000001000101101101  | 43519  | 00001010100111111111  | 193405 | 00101111001101111101 |
| 4637  | 00000001001000011101  | 43557  | 00001010101000100101  | 194543 | 00101111011111101111 |
| 4901  | 0000000100110010101   | 44267  | 00001010110011101011  | 195443 | 00101111101101110011 |
| 5191  | 00000001010001000111  | 44851  | 00001010111100110011  | 210125 | 0011001100011001101  |
| 5225  | 00000001010001101001  | 44877  | 00001010111101001101  | 210677 | 00110011011011110101 |
| 5607  | 00000001010111100111  | 45885  | 00001011001100111101  | 216767 | 00110100111010111111 |
| 6077  | 00000001011110111101  | 46507  | 00001011010110101011  | 219887 | 00110101101011101111 |
| 6371  | 00000001100011100011  | 47407  | 00001011100100101111  | 221183 | 00110101111111111111 |
| 6399  | 00000001100011111111  | 48023  | 00001011101110010111  | 236775 | 00111001110011001111 |
| 6439  | 00000001100100100111  | 48455  | 00001011110101000111  | 241467 | 00111010111100111011 |
| 7009  | 00000001101101100001  | 48693  | 00001011111000110101  | 251639 | 00111101011011110111 |
| 7183  | 00000001110000001111  | 48831  | 00001011111010111111  | 256747 | 00111110101011110101 |
| 7491  | 00000001110101000011  | 49117  | 000010111111111101101 | 261851 | 00111111111011011011 |
| 7637  | 00000001110111010101  | 50105  | 00001100001110111001  | 356191 | 01010110111101011111 |
| 7723  | 00000001111000101011  | 51083  | 00001100011110001011  | 458175 | 01101111110101111111 |
| 8115  | 00000001111110110011  | 51791  | 00001100101001001111  | 489335 | 01110111011101110111 |
| 8719  | 00000010001000001111  | 52135  | 00001100101110100111  | 524287 | 01111111111111111111 |
| 8851  | 00000010001010010011  | 52351  | 00001100110001111111  |        |                      |
| 9225  | 000000100010000001001 | 53037  | 00001100111100101101  |        |                      |
| 9557  | 00000010010101010101  | 53833  | 00001101001001001001  |        |                      |
| 9631  | 00000010010110011111  | 54587  | 00001101010100111011  |        |                      |
| 10199 | 00000010011111010111  | 54997  | 00001101011011010101  |        |                      |
| 10691 | 00000010011110000111  | 55435  | 00001101100010001011  |        |                      |
| 11003 | 00000010101011111011  | 56095  | 00001101101100011111  |        |                      |
| 11097 | 00000010101101011001  | 57083  | 00001101111011111011  |        |                      |
| 11659 | 00000010110110001011  | 58815  | 00001110010110111111  |        |                      |
| 11839 | 00000010111000111111  | 59163  | 00001110011100011011  |        |                      |
| 11909 | 00000010111010000101  | 60109  | 00001110101011001101  |        |                      |
| 12177 | 00000010111110010001  | 60687  | 00001110110100001111  |        |                      |
| 12399 | 00000011000001101111  | 62195  | 00001111001011110011  |        |                      |
| 12587 | 00000011000100101011  | 62289  | 00001111001101010001  |        |                      |
| 12851 | 00000011001000110011  | 63907  | 00001111100110100011  |        |                      |
| 13041 | 00000011001011110001  | 63983  | 00001111100111101111  |        |                      |
| 13243 | 00000011001110110111  | 65195  | 00001111111010101011  |        |                      |
| 13345 | 00000011010000100001  | 65383  | 00001111111101100111  |        |                      |
| 13837 | 00000011011000001101  | 65535  | 00001111111111111111  |        |                      |
| 13999 | 00000011011010101111  | 70895  | 00010001010011101111  |        |                      |
| 14775 | 00000011110011011011  | 71353  | 00010001011010111001  |        |                      |
| 15507 | 00000011110010010011  | 72009  | 00010001100101001001  |        |                      |
| 15773 | 00000011110110011101  | 73431  | 00010001111011010111  |        |                      |
| 16105 | 00000011111011101001  | 73503  | 00010001111100011111  |        |                      |
| 16143 | 00000011111100001111  | 74431  | 00010010001010111111  |        |                      |
| 16985 | 00000100001001011001  | 74867  | 00010010010001110011  |        |                      |
| 17173 | 00000100001100010101  | 77267  | 00010010110111010011  |        |                      |
| 17425 | 00000100010000010001  | 77567  | 00010010111011111111  |        |                      |
| 17639 | 00000100010011100111  | 78151  | 00010011000101000111  |        |                      |
| 18143 | 00000100011011011111  | 78313  | 00010011000111101001  |        |                      |
| 18931 | 00000100100111110011  | 79165  | 00010011010100111101  |        |                      |
| 19875 | 00000100110110100011  | 80483  | 00010011101001100011  |        |                      |
| 19949 | 00000100110111101101  | 80863  | 00010011101111011111  |        |                      |
| 20169 | 00000100111011001001  | 81357  | 00010011110111001101  |        |                      |
| 20683 | 00000101000011001011  | 81703  | 00010011111100100111  |        |                      |
| 20733 | 00000101000011111101  | 81787  | 00010011111101111011  |        |                      |
| 21297 | 000001010001100110001 | 84679  | 00010100101010100011  |        |                      |
| 21587 | 00000101010000101001  | 84983  | 00010100101111110111  |        |                      |
| 21957 | 00000101010111000101  | 85339  | 00010100110101011011  |        |                      |
| 22383 | 00000101011101101111  | 86765  | 00010101001011101101  |        |                      |
| 22625 | 00000101100001100001  | 86891  | 00010101001101101011  |        |                      |
| 22877 | 00000101100101011101  | 87711  | 00010101011010011111  |        |                      |
| 24515 | 00000101111110000111  | 89305  | 000101011110011011001 |        |                      |
| 24863 | 00000110000100011111  | 91119  | 00010110001111101111  |        |                      |
| 24933 | 00000110000101100101  | 93367  | 00010110110010110111  |        |                      |
| 26135 | 00000110011000010111  | 95157  | 00010111001110110101  |        |                      |
| 26249 | 00000110011010001001  | 95357  | 00010111010001111101  |        |                      |
| 26623 | 00000110011111111111  | 101475 | 00011000110001100011  |        |                      |
| 26871 | 00000110100011110111  | 101879 | 00011000110111110111  |        |                      |
| 27015 | 00000110100110001111  | 102013 | 00011000111001111101  |        |                      |
| 28275 | 00000110111001110011  | 103787 | 00011001010101101011  |        |                      |

Table 15. 21-bit codes. Total : 376

|       |                         |       |                        |        |                        |        |                         |
|-------|-------------------------|-------|------------------------|--------|------------------------|--------|-------------------------|
| 7     | 00000000000000000111    | 25889 | 000000110010100100001  | 73623  | 00001000111111010111   | 162019 | 000100111100011100011   |
| 51    | 000000000000000110011   | 25981 | 0000001100101011111101 | 74575  | 0000100100011010001111 | 162367 | 000100111101000111111   |
| 85    | 0000000000000001010101  | 26063 | 0000001100101110011111 | 74991  | 0000100100100111011111 | 163241 | 00010011111010101001    |
| 127   | 000000000000001111111   | 26623 | 0000001100111111111111 | 77003  | 000010010110011001011  | 163475 | 00010011111010010011    |
| 265   | 000000000000100001001   | 27167 | 0000001101010000111111 | 77293  | 000010010110111101101  | 167111 | 000101000110011000111   |
| 335   | 000000000000101001111   | 27625 | 000000110101111101001  | 78165  | 000010011000101010101  | 169695 | 00010100101101101111    |
| 467   | 000000000000111010011   | 27883 | 000000110110011101011  | 79421  | 000010011011000111101  | 169959 | 00010100101111100111    |
| 741   | 000000000001011100101   | 27993 | 000000110110101011001  | 79829  | 00001001101111010101   | 170295 | 000101001100100110111   |
| 771   | 000000000001100000011   | 29007 | 000000111000101001111  | 80599  | 00001001110101101011   | 170909 | 000101001101110011101   |
| 959   | 000000000001110111111   | 29505 | 000000111001101000001  | 81329  | 000010011110110110001  | 171365 | 000101001110101100101   |
| 1187  | 000000000010010100011   | 29607 | 000000111001110100111  | 81549  | 000010011111010001101  | 174059 | 00010100101111101011    |
| 1245  | 00000000001001101101    | 30059 | 000000111010101101011  | 81791  | 000010011111101111111  | 174285 | 000101010100011001101   |
| 1567  | 000000000011000011111   | 30249 | 000000111011000101001  | 82747  | 000010100001100111011  | 175485 | 000101010110101111101   |
| 1927  | 000000000011110000111   | 30753 | 00000011110000100001   | 83155  | 000010100010011010011  | 177499 | 00010101010101011011    |
| 1961  | 000000000011110101001   | 30847 | 000000111100001111111  | 83673  | 000010100011011011001  | 179481 | 000101011110100011001   |
| 2019  | 000000000011111100011   | 31683 | 000000111101111000011  | 84619  | 000010100101010001011  | 180053 | 00010101111101010101    |
| 2263  | 000000000010001101011   | 31909 | 000000111110010100101  | 84665  | 000010100101010111001  | 181723 | 00010100010111011011    |
| 2367  | 000000000010010111111   | 32191 | 000000111110110111111  | 85087  | 000010100110001011111  | 182557 | 000101001001000111001   |
| 2571  | 000000000010100001011   | 32625 | 000000111111101100001  | 85851  | 000010100111101011011  | 186739 | 000101010100010110011   |
| 2833  | 000000000101100010001   | 33425 | 000001000001010010001  | 86259  | 000010101000011110011  | 188215 | 00010101111100110111    |
| 3173  | 00000000010001100101    | 33583 | 000001000001100101111  | 86383  | 00001010100010101111   | 190759 | 00010101010001001011    |
| 3373  | 00000000010100101101    | 34155 | 000001000010101101011  | 88631  | 000010101101000110111  | 190955 | 000101110100111101011   |
| 3535  | 000000000110111011111   | 34707 | 000001000011110010111  | 89679  | 000010101111001001111  | 191417 | 000101110101011011001   |
| 3771  | 000000000111010111011   | 34805 | 000001000011111101011  | 89875  | 00001010111100010011   | 195071 | 000101111100111111111   |
| 4095  | 000000000111111111111   | 35123 | 000001000100100110011  | 90557  | 000010110000110111101  | 195803 | 00010111101011011011    |
| 4283  | 000000001000010111011   | 35703 | 000001000101101110111  | 92313  | 000010110100010011001  | 204267 | 00010000110111101011    |
| 4461  | 000000001000101101101   | 36415 | 000001000111000111111  | 92617  | 000010110100111001001  | 204581 | 00010000111100100101    |
| 4637  | 00000000101000011101    | 37027 | 000001001000010100011  | 92927  | 000010110101011111111  | 207283 | 00010010010101100111    |
| 4901  | 00000000101100101001    | 37301 | 000001001000110110101  | 92963  | 000010110101100100011  | 208557 | 00010010101010101011    |
| 5191  | 000000001010001000111   | 37639 | 000001001001100000111  | 93499  | 000010110110100111011  | 209887 | 000100110011110111111   |
| 5225  | 000000001010001010001   | 38537 | 000001001010100010001  | 94563  | 000010111000101100011  | 210079 | 000100101001001011111   |
| 5607  | 000000001010111100111   | 38851 | 000001001011110000111  | 94797  | 000010111001001001101  | 210169 | 00010011010011111001    |
| 6077  | 000000001011110111101   | 39001 | 000001001100001011001  | 95039  | 000010111001100111111  | 211407 | 000100110100101101111   |
| 6209  | 000000001100001000001   | 39547 | 000001001101001111011  | 95925  | 000010111011010110101  | 214783 | 000101000011011111111   |
| 6371  | 000000001100011100011   | 39571 | 000001001101010010011  | 96227  | 000010111011111000011  | 218447 | 000101010101010100111   |
| 6399  | 000000001100011111111   | 40751 | 000001001111001011111  | 97511  | 000010111100111001111  | 219063 | 00010101011101101111    |
| 6439  | 000000001100100100111   | 41465 | 00000101000011111001   | 97529  | 000010111110011111001  | 219435 | 000101010100100101011   |
| 7009  | 000000001101101100001   | 41613 | 0000010100001010001101 | 100007 | 000011000011010100111  | 222055 | 000101010001101100111   |
| 7183  | 000000001110000001111   | 41951 | 000001010000111101111  | 101021 | 000011000101010011101  | 223981 | 00010101010101101101    |
| 7427  | 000000001110100000011   | 43061 | 000001010100000110101  | 101973 | 000011000111001010101  | 225085 | 000101011111001111101   |
| 7637  | 00000000111011010101    | 43477 | 0000010100101111010101 | 102111 | 000011000111011011111  | 228143 | 000101011110100111111   |
| 7735  | 000000001111000110111   | 43607 | 000001010101001010111  | 103063 | 000011001001010010111  | 233171 | 000110001110110100111   |
| 8115  | 000000001111110110011   | 43919 | 000001010101110001111  | 104443 | 000011001011111111011  | 234991 | 000110001010101110111   |
| 8727  | 000000010001000010111   | 44787 | 000001010111011110011  | 105427 | 000011001101111010011  | 237401 | 00011000111101011001    |
| 8899  | 000000010001010000011   | 45053 | 000001010111111111011  | 106129 | 000011001111010010001  | 238975 | 000110001010101111111   |
| 9221  | 000000010010000000101   | 46755 | 000001011010101000111  | 108339 | 000011010011100110011  | 242171 | 000110110000111110111   |
| 9385  | 000000010010010101001   | 46957 | 000001010110110110101  | 108759 | 000011010100011010111  | 244043 | 000110110100100101011   |
| 9631  | 000000010010110101111   | 47243 | 000001011100010001011  | 108881 | 000011010100101010001  | 244671 | 000110110111011111111   |
| 9707  | 000000010010111101011   | 47721 | 000001011101001101001  | 109553 | 000011010101111110001  | 245225 | 00011011010111101001    |
| 10019 | 000000010011100100101   | 48607 | 000001011110110111111  | 110429 | 000011010111110101101  | 251643 | 000111010101111101101   |
| 10545 | 00000001001100100110001 | 49057 | 000001011111110100001  | 111465 | 000011011001101101001  | 252781 | 00011101101101101101    |
| 10739 | 000000010100111101001   | 49783 | 000001100001001110111  | 111837 | 000011011010011011101  | 255677 | 00011110011010111101    |
| 10917 | 000000010101010100101   | 50765 | 000001100011001001101  | 112891 | 000011011100011111011  | 255911 | 000111100101111010011   |
| 11355 | 000000010110001011011   | 50915 | 000001100011011100011  | 114463 | 000011011111000111111  | 257487 | 000111101011101101111   |
| 11661 | 000000010110110011011   | 51629 | 000001100100110101101  | 117083 | 000011100100101011011  | 260735 | 000111111101001111111   |
| 12025 | 000000010111011111001   | 52327 | 000001100110001100111  | 118165 | 000011100110110010101  | 299593 | 001001001001001001001   |
| 12119 | 000000010111010101111   | 53015 | 000001100111100010111  | 118591 | 000011100111100111111  | 300415 | 001001001010101111111   |
| 12177 | 000000010111110010001   | 53171 | 000001100111110110011  | 119071 | 000011101000100011111  | 303067 | 001001001111110101111   |
| 12351 | 000000011000000111111   | 53627 | 000001101000010111011  | 120613 | 000011101011100100101  | 304293 | 001001001000101010101   |
| 12939 | 000000011001010001011   | 53959 | 000001101001011000111  | 120687 | 000011101011101101111  | 308215 | 001001010111111011111   |
| 13167 | 000000011001101101111   | 54833 | 000001101011000110001  | 121971 | 000011101110001110011  | 314829 | 00100110011011001101    |
| 13363 | 000000011010000110011   | 55157 | 000001101011101110101  | 122199 | 000011101110101010111  | 316763 | 001001101010101010101   |
| 14087 | 000000011011100000111   | 55599 | 000001101100100101111  | 123481 | 000011110001001011001  | 318909 | 001001101101101101101   |
| 14421 | 000000011100001010101   | 56295 | 000001101101111100111  | 123855 | 000011110001111001111  | 325101 | 001001111010111101101   |
| 14577 | 00000001110001110001    | 56517 | 000001101110011000101  | 124139 | 000011110010011101011  | 327653 | 001001111111110010101   |
| 15351 | 000000011101111101111   | 58251 | 000001110001110001011  | 126425 | 000011110110111011001  | 341429 | 001010011010110110101   |
| 15519 | 000000011110010011111   | 58349 | 000001110001111101101  | 126975 | 000011110111111111111  | 349525 | 001010101010101010101   |
| 16099 | 000000011111011100011   | 58425 | 000001110010000111001  | 128275 | 000011111010100010011  | 350639 | 001010101100110101111   |
| 16271 | 000000011111100011111   | 58623 | 000001110010011111111  | 128415 | 000011111010110011111  | 351485 | 001010101100011011101   |
| 16743 | 000000100000101100111   | 58803 | 000001110010110110011  | 128941 | 000011111011111010101  | 354127 | 001010011001110100111   |
| 16801 | 000000100000110100001   | 59601 | 000001110100011010001  | 129237 | 000011111100011010101  | 357567 | 001010111010010111111   |
| 17173 | 000000100001100010101   | 59803 | 000001110100110011011  | 130803 | 000011111111011110011  | 366205 | 001010010100111110101   |
| 17483 | 000000100010001001011   | 60551 | 000001110110010000111  | 130851 | 000011111111100100011  | 375731 | 001011111011001100111   |
| 17529 | 000000100010001111001   | 61055 | 000001110111001111111  | 140119 | 00100001000101010111   | 376575 | 001011011111011111111   |
| 18167 | 000000100011011110111   | 62365 | 000001111001110011101  | 142547 | 00100001011001010011   | 379799 | 001011100101110010111   |
| 18259 | 000000100011101010011   | 62563 | 000001111010001100011  | 143167 | 001000010111100111111  | 383863 | 001011101101101101101   |
| 19119 | 000000100101010101111   | 62797 | 000001111010101001101  | 145203 | 001000011011100110011  | 384975 | 001011101111110011111   |
| 19141 | 000000100101011000101   | 63671 | 000001111100010110111  | 146759 | 001000011101010001111  | 387037 | 0010111100111101101101  |
| 19995 | 000000100111000011011   | 64245 | 000001111101011110101  | 146941 | 001000011110111111101  | 393047 | 001011111111010101111   |
| 20081 | 000000100111001110001   | 64571 | 000001111110000111011  | 148617 | 001001000100100010001  | 421853 | 00110001101111101101101 |
| 20229 | 000000100111100000101   | 65099 | 000001111111001001011  | 149469 | 001001000011110111101  | 425207 | 001100011111001110111   |
| 20599 | 000000101000001110111   | 65499 | 000001111111111101011  | 149989 | 001001001001111001011  | 425983 | 001100011111111111111   |
| 21303 | 000000100100110011011   | 6770  |                        |        |                        |        |                         |
